# Supplementary material for: Detecting Lesion Bounding Ellipses With Gaussian Proposal Networks
Source: arXiv:1902.09658 ancillary file (2019-02-25)
Supplement: Supplementary file 1 [file supplementary.pdf]

# Supplementary for "Detecting Lesion Bounding Ellipses With Gaussian Proposal Networks"

Yi Li

*Baidu Research Institute, 1195 Bordeaux Dr. Sunnyvale, CA 94089*

## 1 KL divergence of 2D Gaussian distributions

In this section, we provide the mathematical details of deriving Equation 10 through Equation 12 in the main manuscript of the KL divergence between 2D Gaussian distributions. Following Equation 8 in the main manuscript, we use a 2D Gaussian distribution in the $(x, y)$ system parameterized by

$$\boldsymbol{\mu} = \begin{bmatrix}\mu_x \\ \mu_y\end{bmatrix}, \boldsymbol{\Sigma}^{-1} = R^\intercal(\theta)\begin{bmatrix}\frac{1}{\sigma_l^2} & 0 \\ 0 & \frac{1}{\sigma_s^2}\end{bmatrix}R(\theta), R(\theta) = \begin{bmatrix}\cos\theta & \sin\theta \\ -\sin\theta & \cos\theta\end{bmatrix}, \tag{1}$$

to represent the ellipse centered at $(\mu_x, \mu_y)$, with semi-major and semi-minor axises of lengths $(\sigma_l, \sigma_s)$, and a rotation angle of $\theta$ between its major axis and the $x$ axis.

We first take the inverse of $\boldsymbol{\Sigma}^{-1}$ to obtain $\boldsymbol{\Sigma}$. Because $R(\theta)$ is orthogonal, we have

$$R^\intercal(\theta) = R^{-1}(\theta) = R(-\theta). \tag{2}$$

Expanding $\boldsymbol{\Sigma}^{-1}$, we have

$$\begin{aligned}\boldsymbol{\Sigma}^{-1} &= R^\intercal(\theta)\begin{bmatrix}\frac{1}{\sigma_l^2} & 0 \\ 0 & \frac{1}{\sigma_s^2}\end{bmatrix}R(\theta) \\ &= \begin{bmatrix}\cos\theta & -\sin\theta \\ \sin\theta & \cos\theta\end{bmatrix}\begin{bmatrix}\frac{1}{\sigma_l^2} & 0 \\ 0 & \frac{1}{\sigma_s^2}\end{bmatrix}\begin{bmatrix}\cos\theta & \sin\theta \\ -\sin\theta & \cos\theta\end{bmatrix} \\ &= \begin{bmatrix}\frac{\cos^2\theta}{\sigma_l^2} + \frac{\sin^2\theta}{\sigma_s^2} & \frac{\sin\theta\cos\theta}{\sigma_l^2} - \frac{\sin\theta\cos\theta}{\sigma_s^2} \\ \frac{\sin\theta\cos\theta}{\sigma_l^2} - \frac{\sin\theta\cos\theta}{\sigma_s^2} & \frac{\sin^2\theta}{\sigma_l^2} + \frac{\cos^2\theta}{\sigma_s^2}\end{bmatrix}.\end{aligned} \tag{3}$$

Then, we can derive the determinant and the adjugate of $\boldsymbol{\Sigma}^{-1}$ as

$$\begin{aligned}|\boldsymbol{\Sigma}^{-1}| &= \frac{1}{\sigma_l^2\sigma_s^2}, \\ \text{adj}(\boldsymbol{\Sigma}^{-1}) &= \begin{bmatrix}\frac{\cos^2\theta}{\sigma_s^2} + \frac{\sin^2\theta}{\sigma_l^2} & \frac{\sin\theta\cos\theta}{\sigma_s^2} - \frac{\sin\theta\cos\theta}{\sigma_l^2} \\ \frac{\sin\theta\cos\theta}{\sigma_s^2} - \frac{\sin\theta\cos\theta}{\sigma_l^2} & \frac{\sin^2\theta}{\sigma_s^2} + \frac{\cos^2\theta}{\sigma_l^2}\end{bmatrix}.\end{aligned} \tag{4}$$

Finally, we can derive $\boldsymbol{\Sigma}$ as

$$\begin{aligned}\boldsymbol{\Sigma} &= \frac{\text{adj}(\boldsymbol{\Sigma}^{-1})}{|\boldsymbol{\Sigma}^{-1}|} \\ &= \begin{bmatrix}\cos^2\theta\ \sigma_l^2 + \sin^2\theta\ \sigma_s^2 & \sin\theta\cos\theta\ \sigma_l^2 - \sin\theta\cos\theta\ \sigma_s^2 \\ \sin\theta\cos\theta\ \sigma_l^2 - \sin\theta\cos\theta\ \sigma_s^2 & \sin^2\theta\ \sigma_l^2 + \cos^2\theta\ \sigma_s^2\end{bmatrix} \\ &= R^\intercal(\theta)\begin{bmatrix}\sigma_l^2 & 0 \\ 0 & \sigma_s^2\end{bmatrix}R(\theta),\end{aligned} \tag{5}$$

where $R(\theta)$ is the same rotation matrix defined above. The determinant of $\boldsymbol{\Sigma}$ is given as

$$|\boldsymbol{\Sigma}| = \sigma_l^2\sigma_s^2. \tag{6}$$

Now we derive the full expression of the KL divergence between a proposed 2D Gaussian distribution $\mathcal{N}_p$ and a target 2D Gaussian distribution $\mathcal{N}_t$ [1]:

$$D_{\text{KL}}(\mathcal{N}_t||\mathcal{N}_p) = \frac{1}{2}\left[\text{tr}(\boldsymbol{\Sigma}_p^{-1}\boldsymbol{\Sigma}_t) + (\boldsymbol{\mu}_p - \boldsymbol{\mu}_t)^\intercal\boldsymbol{\Sigma}_p^{-1}(\boldsymbol{\mu}_p - \boldsymbol{\mu}_t) + \ln\frac{|\boldsymbol{\Sigma}_p|}{|\boldsymbol{\Sigma}_t|} - 2\right]. \tag{7}$$

We parameterize $\mathcal{N}_p$ and $\mathcal{N}_t$ by $(\mu_{x_p}, \mu_{y_p}, \sigma_{l_p}, \sigma_{s_p}, \theta_p)$ and $(\mu_{x_t}, \mu_{y_t}, \sigma_{l_t}, \sigma_{s_t}, \theta_t)$. Then, for the trace we have

$$\begin{aligned}
\mathrm{tr}(\boldsymbol{\Sigma}_p^{-1}\boldsymbol{\Sigma}_t) =&\mathrm{tr}\left(R^\intercal(\theta_p)\begin{bmatrix}\frac{1}{\sigma_{l_p}^2} & 0\\ 0 & \frac{1}{\sigma_{s_p}^2}\end{bmatrix}R(\theta_p)R^\intercal(\theta_t)\begin{bmatrix}\sigma_{l_t}^2 & 0\\ 0 & \sigma_{s_t}^2\end{bmatrix}R(\theta_t)\right)\\
=&\mathrm{tr}\left(R(\theta_t)R^\intercal(\theta_p)\begin{bmatrix}\frac{1}{\sigma_{l_p}^2} & 0\\ 0 & \frac{1}{\sigma_{s_p}^2}\end{bmatrix}R(\theta_p)R^\intercal(\theta_t)\begin{bmatrix}\sigma_{l_t}^2 & 0\\ 0 & \sigma_{s_t}^2\end{bmatrix}\right)\\
=&\mathrm{tr}\left(R^\intercal(\theta_p-\theta_t)\begin{bmatrix}\frac{1}{\sigma_{l_p}^2} & 0\\ 0 & \frac{1}{\sigma_{s_p}^2}\end{bmatrix}R(\theta_p-\theta_t)\begin{bmatrix}\sigma_{l_t}^2 & 0\\ 0 & \sigma_{s_t}^2\end{bmatrix}\right)\\
=&\cos^2\Delta\theta\ \frac{\sigma_{l_t}^2}{\sigma_{l_p}^2}+\cos^2\Delta\theta\ \frac{\sigma_{s_t}^2}{\sigma_{s_p}^2}+\sin^2\Delta\theta\ \frac{\sigma_{l_t}^2}{\sigma_{s_p}^2}+\sin^2\Delta\theta\ \frac{\sigma_{s_t}^2}{\sigma_{l_p}^2}.
\end{aligned} \tag{8}$$

where we have used trace invariance under cyclic permutations and we define $\Delta\theta = \theta_p - \theta_t$.

For the Mahalanobis distance, we have

$$\begin{aligned}
(\boldsymbol{\mu}_p-\boldsymbol{\mu}_t)^\intercal\boldsymbol{\Sigma}_p^{-1}(\boldsymbol{\mu}_p-\boldsymbol{\mu}_t) =&\begin{bmatrix}\mu_{x_p}-\mu_{x_t}\\ \mu_{y_p}-\mu_{y_t}\end{bmatrix}^\intercal R^\intercal(\theta_p)\begin{bmatrix}\frac{1}{\sigma_{l_p}^2} & 0\\ 0 & \frac{1}{\sigma_{s_p}^2}\end{bmatrix}R(\theta_p)\begin{bmatrix}\mu_{x_p}-\mu_{x_t}\\ \mu_{y_p}-\mu_{y_t}\end{bmatrix}\\
=&\left(R(\theta_p)\begin{bmatrix}\Delta x\\ \Delta y\end{bmatrix}\right)^\intercal\begin{bmatrix}\frac{1}{\sigma_{l_p}^2} & 0\\ 0 & \frac{1}{\sigma_{s_p}^2}\end{bmatrix}\left(R(\theta_p)\begin{bmatrix}\Delta x\\ \Delta y\end{bmatrix}\right)\\
=&\frac{(\cos\theta_p\Delta x+\sin\theta_p\Delta y)^2}{\sigma_{l_p}^2}+\frac{(\cos\theta_p\Delta y-\sin\theta_p\Delta x)^2}{\sigma_{s_p}^2},
\end{aligned} \tag{9}$$

where we define $\Delta x = \mu_{x_p} - \mu_{x_t}$, $\Delta y = \mu_{y_p} - \mu_{y_t}$.

For the determinant, we have

$$\ln\frac{|\boldsymbol{\Sigma}_p|}{|\boldsymbol{\Sigma}_t|} = \ln\frac{\sigma_{l_p}^2}{\sigma_{l_t}^2} + \ln\frac{\sigma_{s_p}^2}{\sigma_{s_t}^2}. \tag{10}$$

# 2 Data preprocessing

We follow the practices from [4] to convert the raw slice images with pixel value in Hounsfield Unit (HU) into 512×512 three channel images with pixel values between 0 and 255. Specifically, we clip the HU values into range of $[-1024, 3071]$, and then normalize them into $[0, 255]$. Both images and their two axises annotations are resized such that each pixel on the image plane corresponds to 0.8 mm in physical scale. If the resized image is smaller than 512×512, we pad on its border with pixel value of 50, which is the value we use for pixel mean subtraction during training. If the resized image is larger than 512×512, we further resize it back to 512×512. Therefore, the final input image to the network has a fixed size of 512×512. Slice intervals on the z-axis (vertical), are linearly interpolated into 2 mm. Three consecutive slices, with the middle one containing the two axises annotation, are stacked vertically to make a three channel image.

Bounding ellipses are generated from the two axises annotations. Specifically, the lengths of the major and minor axises from the annotation are used as the lengths of the major and minor axises of the bounding ellipse. The rotation angle and the center of the major axis from the annotation are used as the rotation angle and the center of the bounding ellipse. We note this setting may introduce inaccurate representation of the two axises annotation, but we think it is minor as we have discussed in the main manuscript.

# 3 Model training and evaluation

We use the official split from DeepLesion for training (70%), validation (15%), and test (15%). All the networks are trained with 20 epochs. The learning rate for the first 10 epochs is 0.001 and decreased by 0.1 for the second 10 epochs. The model with the highest average free-response receiver operating characteristic (FROC) score on the validation set is saved as the best model for performance evaluation. The average FROC score is defined as the average detection sensitivity at 6 predefined false positives per image: 0.5, 1, 2, 4, 8 and 16. Momentum of 0.9, gradient clipping of 10.0 and weight decay of 0.0005 are applied during training. Each batch is composed of 2 images and each image generates 32 proposals during training.

We compute intersection over union (IoU) between ellipses by rasterizing ellipses first and then counting the pixel overlaps. However this numerical approach is compute intensive, therefore we only use it for performance evaluation. During training, we use the bounding box that tightly surrounds the bounding ellipse to compute IoU for anchor assignment and non-maximum suppression (NMS). We use the standard practices from RPN [3] to assign anchors, Specifically, anchors with the largest

IoU and IoU greater than 0.7 with the ground truth are assigned with positive labels. Anchors with IoU less than 0.3 are assigned with negative labels. We keep the top 6000 proposals before NMS and the top 300 proposals after NMS for each image during inference time.

# 4 Comparison between Softer-NMS and GPN

The recent Softer-NMS [2] also uses KL divergence for bounding box localization. However, the main purpose of Softer-NMS is to model the location uncertainty of proposed bounding boxes. Therefore, Softer-NMS uses a 1D Gaussian to model the location distributions of top left and bottom right corners of proposed bounding boxes. It also introduces another trainable parameter $\sigma$ to characterize the 1D Gaussian. For ground truth bounding boxes, Softer-NMS uses Dirac delta distribution to model the location distribution since it does not have uncertainty. Softer-NMS then optimizes the KL divergence between the 1D Gaussian and the Dirac delta distribution for object localization. On the other hand, the main purpose of GPN is to propose bounding ellipses, therefore it is not directly comparable to Softer-NMS. When assuming the rotation angle is 0, the bounding ellipse may be viewed as a bounding box characterized by the major and minor axises of the bounding ellipse. Yet, instead of modeling the location uncertainty of bounding box corners, GPN views both the proposed bounding box and the ground truth bounding box themselves as 2D Gaussian distributions and optimize their KL divergence for localization.

# 5 Rotation angle error on the test set

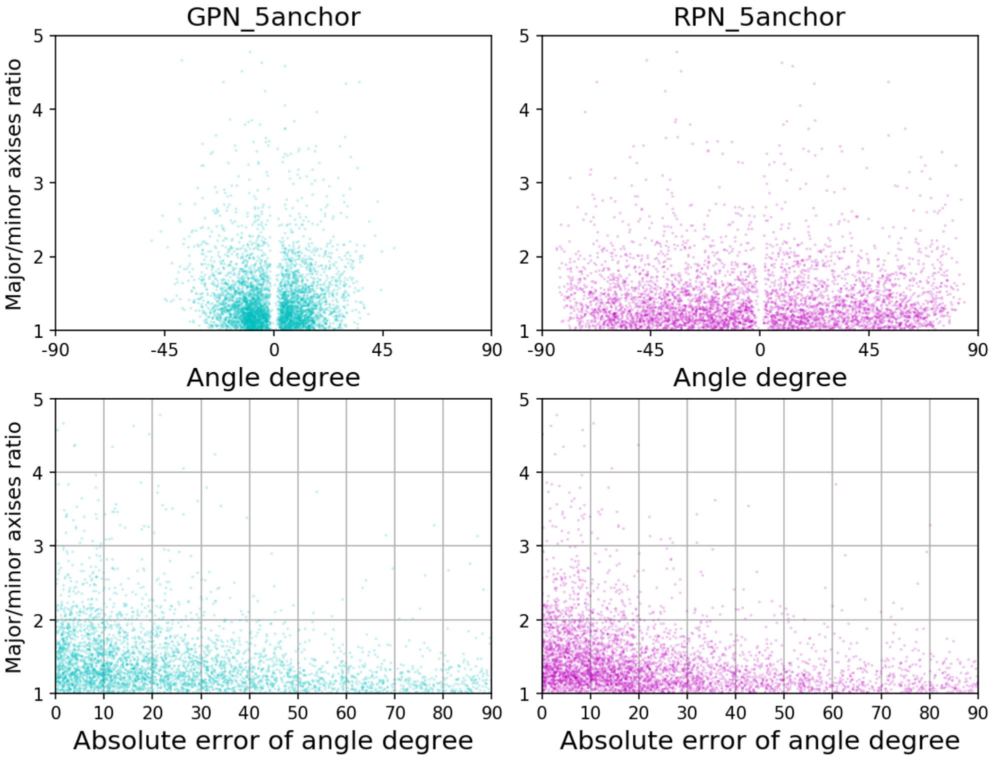


Figure 1: **The upper panels** are the distributions of predicted angles of GPN-5anchor and RPN-5anchor with respect to the ground truth aspect ratio on the test set of DeepLesion. **The lower panels** are the absolute degree errors of predicted angles of GPN-5anchor and RPN-5anchor with respect to the ground truth aspect ratio on the test set of DeepLesion.

# References


[1] J. Duchi. Derivations for linear algebra and optimization. *Berkeley, California*, 3, 2007.

[2] Y. He, X. Zhang, M. Savvides, and K. Kitani. Softer-nms: Rethinking bounding box regression for accurate object detection. *arXiv preprint arXiv:1809.08545*, 2018.

[3] S. Ren, K. He, R. Girshick, and J. Sun. Faster r-cnn: Towards real-time object detection with region proposal networks. In *Advances in neural information processing systems*, pages 91–99, 2015.

[4] K. Yan, M. Bagheri, and R. M. Summers. 3d context enhanced region-based convolutional neural network for end-to-end lesion detection. In *International Conference on Medical Image Computing and Computer-Assisted Intervention*, pages 511–519. Springer, 2018.
